# Supplementary material for: Factual Probing Is [MASK]: Learning vs. Learning to Recall
Source: arXiv:2104.05240 source file (2021-12-14)
Supplement: Supplementary file 1 [file naacl2021-submission-appendix.pdf]

## A Breakdown Accuracy for LAMA

In Table 5, we show a detailed breakdown of per-relation probing accuracy as well as their control accuracy and class prior on the LAMA test set.

## B Implementation Details

We implement OPTIPROMPT based on the HuggingFace’s Transformers (Wolf et al., 2020) library. During training, we use an Adam optimizer and a scheduler with a warmup ratio of 0.1. We use an Adam optimizer and a linear scheduler with a warmup ratio of 0.1. We train our OPTIPROMPT model for 10 epochs with a learning rate of  $3e - 3$  and a batch size of 16. For fine-tuning, we use an Adam optimizer and a linear scheduler with a warmup ratio of 0.1. We fine-tune the language models for 10 epochs with a learning rate of  $2e - 6$  and a batch size of 2.

We report AUTOPROMPT’s performance based on the prompts released by Shin et al. (2020). When we apply AUTOPROMPT to a control task (e.g., the Random Embeddings model), or compare AUTOPROMPT with different language models on a different dataset (see Appendix C), we run AUTOPROMPT for 1000 iterations for each model to search for the prompt of a relation.

## C Comparing Pre-trained Language Models

We compare different pre-trained language models with different probing methods. We collect at most 1000 training samples for each relation from the TRE-x dataset and constrain the object of each sample to be a token for all the models<sup>6</sup>. During testing, we downsample the LAMA test set to make sure that the object in each sample is a single token for all the models. In Table 6 shows the results of different probing methods applied to four pre-trained language models, along with our Random Model baseline. We make the following observations:

- **Base vs. Large:** The larger version of BERT performs better on LAMA than BERT base in both OPTIPROMPT and fine-tuning probes. We might hypothesize that BERT-large is simply more capable of finding patterns in the training data, but our baseline result does not

indicate that this is the case—on the contrary, BERT-large performs marginally worse on the Random Model baseline. This could lead us to believe that BERT-large truly does store information about 1 or 2% more LAMA facts compared to BERT-base.

- **BERT vs. RoBERTa vs. ALBERT:** Shin et al. (2020) find that RoBERTa performs significantly worse on LAMA than BERT. We find this is true for our prompts as well (comparing with BERT-large), but the magnitude of the difference decreases in the fine-tuning setting. Our baseline result gives a possible hint as to why: RoBERTa performs better on the control task with fine-tuning, indicating that part of the difference between OPTIPROMPT and fine-tuning might be due to better exploitation of training data. This change is even more dramatic in ALBERT. Perhaps these models store less factual information due to pre-training on a wider variety of genres.

We believe that further comparisons along these lines are a promising area of future work—for example, if we could show that probing results are correlated with downstream task performance and use probes to guide model selection.

<sup>6</sup>The original data collected by Shin et al. (2020) is not applicable when we compare different language models, because some object tokens are not in the vocabulary of RoBERTa or ALBERT

| Relation | LAMA (manual prompts)                         |      | OPTIPROMPT |         |         | Fine-tuning |         |         | Class Prior |
|----------|-----------------------------------------------|------|------------|---------|---------|-------------|---------|---------|-------------|
|          | Prompt                                        | Acc  | Acc        | Rand E. | Rand M. | Acc         | Rand E. | Rand M. |             |
| P1001    | [X] is a legal term in [Y] .                  | 70.5 | 85.5       | 50.4    | 9.4     | 85.5        | 53.9    | 9.6     | 9.6         |
| P101     | [X] works in the field of [Y] .               | 9.9  | 13.4       | 8.9     | 10.1    | 15.2        | 11.5    | 10.8    | 10.8        |
| P103     | The native language of [X] is [Y] .           | 72.2 | 85.8       | 60.0    | 60.0    | 87.3        | 63.7    | 60.1    | 60.1        |
| P106     | [X] is a [Y] by profession .                  | 0.6  | 37.0       | 30.0    | 20.7    | 33.4        | 29.1    | 25.6    | 14.3        |
| P108     | [X] works for [Y] .                           | 6.8  | 9.7        | 7.3     | 7.3     | 10.4        | 7.3     | 7.8     | 7.8         |
| P127     | [X] is owned by [Y] .                         | 34.8 | 51.4       | 7.1     | 10.2    | 52.6        | 17.2    | 14.7    | 6.8         |
| P1303    | [X] plays [Y] .                               | 7.6  | 24.9       | 22.8    | 22.3    | 24.9        | 22.8    | 22.8    | 22.8        |
| P131     | [X] is located in [Y] .                       | 23.3 | 39.6       | 0.6     | 1.6     | 40.5        | 1.8     | 0.6     | 0.6         |
| P136     | [X] plays [Y] music .                         | 0.8  | 64.8       | 55.4    | 55.4    | 62.6        | 54.8    | 55.4    | 55.4        |
| P1376    | [X] is the capital of [Y] .                   | 73.9 | 62.7       | 0.9     | 0.0     | 66.5        | 0.0     | 0.4     | 0.4         |
| P138     | [X] is named after [Y] .                      | 61.6 | 74.6       | 0.9     | 0.5     | 73.8        | 35.4    | 1.6     | 1.6         |
| P140     | [X] is affiliated with the [Y] religion .     | 0.6  | 77.6       | 53.7    | 53.7    | 80.1        | 53.7    | 53.7    | 53.7        |
| P1412    | [X] used to communicate in [Y] .              | 65.0 | 76.8       | 25.4    | 20.6    | 76.1        | 27.4    | 26.7    | 20.6        |
| P159     | The headquarter of [X] is in [Y] .            | 32.4 | 37.5       | 9.0     | 9.0     | 37.5        | 9.3     | 9.0     | 9           |
| P17      | [X] is located in [Y] .                       | 31.3 | 57.9       | 3.1     | 2.4     | 58.3        | 7.4     | 2.7     | 2.8         |
| P176     | [X] is produced by [Y] .                      | 85.6 | 87.2       | 8.9     | 8.9     | 90.1        | 82.6    | 68.4    | 8.9         |
| P178     | [X] is developed by [Y] .                     | 62.8 | 68.7       | 8.6     | 4.7     | 61.6        | 33.7    | 8.1     | 4.9         |
| P19      | [X] was born in [Y] .                         | 21.1 | 20.5       | 5.6     | 5.6     | 18.9        | 4.5     | 6.3     | 6.2         |
| P190     | [X] and [Y] are twin cities .                 | 2.4  | 3.1        | 2.6     | 1.3     | 3.1         | 2.5     | 2.1     | 2.7         |
| P20      | [X] died in [Y] .                             | 27.9 | 33.3       | 10.5    | 10.9    | 33.2        | 12.8    | 13.2    | 10.3        |
| P264     | [X] is represented by music label [Y] .       | 9.6  | 47.1       | 37.5    | 37.5    | 50.4        | 37.5    | 37.5    | 37.5        |
| P27      | [X] is [Y] citizen .                          | 0.0  | 47.1       | 10.0    | 5.0     | 49.4        | 11.5    | 10.0    | 10          |
| P276     | [X] is located in [Y] .                       | 41.5 | 47.2       | 5.0     | 4.5     | 49.4        | 5.1     | 4.9     | 4.7         |
| P279     | [X] is a subclass of [Y] .                    | 30.7 | 66.0       | 28.1    | 16.0    | 66.4        | 42.8    | 16.0    | 16          |
| P30      | [X] is located in [Y] .                       | 25.4 | 89.5       | 72.3    | 72.3    | 92.4        | 72.3    | 72.3    | 72.3        |
| P31      | [X] is a [Y] .                                | 36.7 | 65.7       | 8.9     | 8.7     | 69.1        | 28.5    | 9.0     | 8.9         |
| P36      | The capital of [X] is [Y] .                   | 62.2 | 62.0       | 0.0     | 0.0     | 62.8        | 0.6     | 0.0     | 0.1         |
| P361     | [X] is part of [Y] .                          | 23.6 | 46.8       | 6.0     | 6.0     | 48.5        | 7.4     | 6.0     | 6           |
| P364     | The original language of [X] is [Y] .         | 44.5 | 50.0       | 24.9    | 19.7    | 51.9        | 27.0    | 25.6    | 25.1        |
| P37      | The official language of [X] is [Y] .         | 54.6 | 61.4       | 17.0    | 17.0    | 64.7        | 18.0    | 17.0    | 17          |
| P39      | [X] has the position of [Y] .                 | 8.0  | 43.4       | 31.4    | 31.4    | 42.2        | 33.7    | 29.5    | 27.2        |
| P407     | [X] was written in [Y] .                      | 59.2 | 70.1       | 46.4    | 46.6    | 72.1        | 46.4    | 46.4    | 46.4        |
| P413     | [X] plays in [Y] position .                   | 0.5  | 43.8       | 41.7    | 41.7    | 41.7        | 41.7    | 41.7    | 41.7        |
| P449     | [X] was originally aired on [Y] .             | 20.9 | 35.2       | 29.7    | 32.5    | 35.2        | 26.8    | 29.2    | 32.6        |
| P463     | [X] is a member of [Y] .                      | 67.1 | 62.7       | 38.2    | 2.2     | 62.2        | 59.1    | 57.3    | 2.2         |
| P47      | [X] shares border with [Y] .                  | 13.7 | 22.3       | 0.0     | 0.0     | 21.9        | 0.4     | 1.1     | 0.3         |
| P495     | [X] was created in [Y] .                      | 16.5 | 40.4       | 10.9    | 11.9    | 39.8        | 14.1    | 13.1    | 10.9        |
| P527     | [X] consists of [Y] .                         | 11.1 | 34.8       | 17.4    | 8.6     | 35.4        | 11.8    | 17.1    | 17.4        |
| P530     | [X] maintains diplomatic relations with [Y] . | 2.8  | 3.3        | 0.4     | 0.6     | 2.9         | 2.4     | 0.7     | 1.1         |
| P740     | [X] was founded in [Y] .                      | 7.6  | 16.7       | 7.4     | 7.4     | 16.0        | 7.3     | 7.4     | 7.4         |
| P937     | [X] used to work in [Y] .                     | 29.8 | 44.4       | 14.8    | 14.8    | 44.6        | 17.4    | 14.8    | 14.8        |

Table 5: A detailed breakdown of per-relation probing accuracy and control accuracy on the LAMA test set. *Rand. E.*: only the input embeddings are randomly initialized. *Rand. M.*: all the weights are randomly initialized. Class Prior is the accuracy from predicting the class that appeared most often in the training data.

| Method      | BERT (110M) |         | BERT (330M) |         | RoBERTa (330M) |         | ALBERT (235M) <sup>†</sup> |         |
|-------------|-------------|---------|-------------|---------|----------------|---------|----------------------------|---------|
|             | Pre-T.      | Rand M. | Pre-T.      | Rand M. | Pre-T.         | Rand M. | Pre-T.                     | Rand M. |
| Manual      | 30.6        | -       | 32.2        | -       | 23.6           | -       | 27.4                       | -       |
| LPAQA       | 35.6        | -       | 36.2        | -       | 29.3           | -       | 29.8                       | -       |
| AUTOPROMPT  | 44.6        | 0.0     | 44.5        | 0.1     | 38.6           | 0.0     | 33.2                       | 0.0     |
| OPTIPROMPT  | 50.8        | 19.9    | 52.7        | 19.3    | 47.8           | 19.6    | 44.6                       | 16.9    |
| Fine-tuning | 51.9        | 19.8    | 54.9        | 19.6    | 52.3           | 21.4    | 52.8                       | 21.1    |

Table 6: Comparison of different pre-trained LMs. We downsample the LAMA test set to make sure that in each sample, the object is a single token for all the models. <sup>†</sup>: there is parameter sharing in ALBERT models so the actual models are much bigger. *Pre-T.*: pre-trained language models. *Rand M.*: randomly initialized models.
